# Supplementary material for: Grounding-Prompter: Prompting LLM with Multimodal Information for Temporal Sentence Grounding in Long Videos
Source: arXiv:2312.17117 source file (2023-12-28)
Supplement: Supplementary file 1 [file X_suppl.tex]

\clearpage
\setcounter{page}{1}
\maketitlesupplementary

\section{Appendix}
